# Supplementary material for: Ordering of Binary Colloidal Crystals by Random Potentials
Source: arXiv:1903.01579 ancillary file (2019-03-04)
Supplement: Supplementary file 1 [file SI.pdf]

# Ordering of Binary Colloidal Crystals by Random Potentials
## Supplementa Material

André S. Nunes,[1,*] Sabareesh K. P. Velu,[2,*] Iryna Kasianiuk,[3] Denys Kasyanyuk,[3] Agnese Callegari,[3] Giorgio Volpe,[4] Margarida M. Telo da Gama,[1] Giovanni Volpe,[2,5] and Nuno A. M. Araújo[1,†]

[1] *Centro de Física Teórica e Computacional and Departamento de Física, Faculdade de Ciências, Universidade de Lisboa, P-1749-016 Lisboa, Portugal, EU*
[2] *Department of Physics, Bilkent University, Cankaya, 06800 Ankara, Turkey*
[3] *Department of Physics, Bilkent University and UNAM, Cankaya, 06800 Ankara, Turkey*
[4] *Department of Chemistry, University College London, 20 Gordon Street, London WC1H 0AJ, United Kingdom, EU*
[5] *Department of Physics, University of Gothenburg, 41296 Gothenburg, Sweden, EU*

### SAMPLE PREPARATION

Diluted aqueous stock solutions of polystyrene and silica colloidal spheres (Microparticles GmbH, diameter $d_{\mathrm{PS}} = 4.06 \pm 0.11\,\mu$m and $d_{\mathrm{SiO_2}} = 3.93 \pm 0.12\,\mu$m, respectively) were used to prepare binary solutions with different molar fractions of polystyrene particles from $\chi = 0$ to $\chi = 1$. The total density of particles was kept constant at $1.4 \cdot 10^7\,\mathrm{mL}^{-1}$. These colloidal solutions were confined in a homemade sample chamber (internal thickness $200\,\mu$m), built between a bottom glass slide (made hydrophilic by treatment in a 0.25 M NaOH solution) and a top flat-terminated fibre coupler (Thorlabs, SM1SMA) held apart by two layers of a thermoplastic spacer, which at the same time was also used for sealing the chamber. The fibre coupler was used to connect the output end of a multimode optical fiber (core diameter 105 m, NA = 0.22, length 1 m) . See also Fig. S1.

### EXPERIMENTAL SETUP

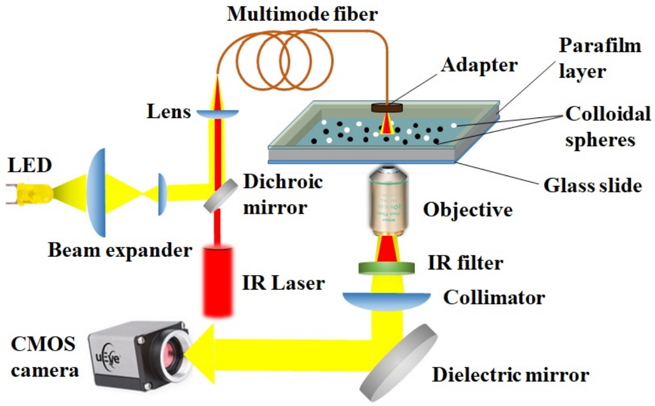


Supplementary Figure S1. Schematic representation of the experimental setup and sample chamber.

A homemade inverted optical microscope setup was used for carrying out the experimental investigations of structural defects in colloidal crystals formed under random optical potentials, as schematically shown in Fig. S1 [1]. An image of the sample with colloidal particles was projected by a microscope objective (Nikon Plan Fluorite Imaging Objective, 20×, NA = 0.5, WD = 2.1 mm) onto a monochrome charge-coupled device (CCD) camera with an acquisition rate between 1 and 8 frames per second (fps). The incoherent illumination was provided by a LED lamp at $\lambda = 625$ nm coupled into the optical fiber using a dichroic mirror (Thorlabs, DMLP605). The particles were tracked by digital video microscopy [2].

The static speckle light pattern with a Gaussian envelope was generated by focusing a laser beam (wavelength $\lambda = 976$ nm, output power $P = 180$ mW) into a multimode optical fiber using a plano-convex lens (focal distance $f = 25.4$ mm). The output speckle pattern is the result of the multipath interference of the optical waves carrying random phases within the multimode optical fiber [1, 3, 4]. The length of the optical path between the fiber tip and the imaging plane where the colloidal particles lay (i.e., the bottom of the sample chamber) determines the final speckle grain size. The typical duration of an experiment is about 90 minutes.

### SIMULATIONS

We performed Brownian dynamics (BD) simulations of a binary mixture of $N = 800$ particles with several compositions, on a two-dimensional square box with periodic boundary conditions and linear size $L$. The particle species differ in the strength of their response to the optical potential. The interaction potential between a pair of particles $i$ and $j$ with diameter $d_p$ is independent of the species and is given by the repulsive part of a Lennard-Jones potential:

$$V_{ij}(r) = \epsilon \left[ \left( \frac{d_p}{r} \right)^{12} - \left( \frac{d_p}{r} \right)^{6} \right], \tag{1}$$

where $\epsilon$ sets the energy scale. This is a very steep and short-ranged potential that only affects neighbouring particles within a cut-off distance of $r_{\mathrm{cut}} = 2^{-1/6} d_p$.

The external potential has two contributions. The first contribution is a Gaussian potential that attracts the particles towards the centre of the simulation box, given by

$$V_{\text{Gaussian}}(r) = \begin{cases} -V_{\text{G}_k} e^{-\frac{(r-7.5)^2}{\sigma_{\text{G}}^2}} & \text{if } r > 7.5 \\ 0 & \text{if } r \leq 7.5 \end{cases} \quad (2)$$

where $\sigma$ is the width of the Gaussian and $V_{\text{G}_k}$ sets the scale of this interaction, which depends on the particle type $k$; the interaction $V_{\text{G}_k}$ with the most responsive (strong) particles is $2\times$ that with the least responsive (weak) ones; $r$ is the distance to the centre of the simulation box. By definition, we ensure that the Gaussian potential is zero in the central region of the box, of radius 7.5, where we carried out the statistical analysis of the system. This potential is used to confine the particles in the centre of the box at sufficiently high densities. The second contribution to the external potential reproduces the potential generated by a speckle pattern [5]. We used the Fourier filtering method (FFM) to generate numerically random potentials with Gaussian spatial correlations [6, 7]. The FFM takes advantage of the fact that the correlation function of a field $E(\vec{r})$, is the inverse Fourier transform of the absolute value of its Fourier coefficients, $|E_{\vec{k}}|^2$, as stated by the Wiener-Khinchin theorem [8]. This relation allows us to sample random Fourier coefficients that when transformed back into real space describe a random potential with the desired spatial correlations. The depths of those potentials have a Gaussian distribution. To convert it into an exponential distribution, as measured for the speckle, we used the following procedure: the random surface is discretized in $1024 \times 1024$ cells, which we sort by the intensity of the potential. Then, we produce a sorted list of intensities drawn from an exponential distribution and substitute each cell intensity by the corresponding entry on the ranked list of intensities. We tested this procedure with Gaussian and power-law correlation functions and confirmed that it does lead to the desired distribution of intensities, without affecting the nature of the correlation function. The forces due to this potential are then calculated using finite differences. In all simulations, we considered Gaussian correlations with a dispersion $\sigma$. When $\sigma < d_{\text{p}}$ (where $d_{\text{p}}$ is the diameter of the particles) the speckle features vary on distances shorter than the particle size and we need to consider an effective speckle pattern that is the result of the integration of the speckle intensities over the particle volume (see below section "Effective speckle properties"). The potentials strength ratio is $V_{\text{G}}/V_{\text{sp}} = 1$ in the simulations presented in Figs. 1, 2, 4(a) and 4(b).

The motion of a particle $i$ in the surrounding medium is described by the overdamped Langevin equation

$$\gamma \frac{d\vec{r}_i}{dt} = -\vec{\nabla}_i \left[ \sum_j V_{ij}(r) + V_{\text{ext}}(\vec{r}_i) \right] + \vec{\xi}_i, \quad j \neq i, \quad (3)$$

where $\gamma$ is the Stokes-Einstein friction coefficient and $\vec{\xi}_i$ is a random stochastic term that mimics the thermal noise that results from the interaction with the medium. This term is given by a normal distribution with zero mean and auto-correlation that is independent of space and time and proportional to the thermostat temperature $T$, i.e. $\left\langle \xi_i^n(t) \xi_i^l(t') \right\rangle = 2 k_{\text{B}} T \gamma_i \delta_{nl} \delta(t-t')$, where $n$ and $l$ are indices that run over the space dimensions and $k_{\text{B}}$ is the Boltzmann constant. The characteristic time is defined as $\tau = d_p^2 \gamma / k_{\text{B}} T$. Equation (3) is integrated following the algorithm developed by Branka and Heyes [9], i.e. a second-order stochastic Runge-Kutta scheme, with a time step of $\Delta t = 10^{-4}\tau$. We set the diameter of the particle, $d_{\text{p}}$, as the unit length, the simulation box has linear size $L = 50$ and the width of the external Gaussian potential is $\sigma_{\text{G}} = L/2$. The energy is given in units of $k_{\text{B}}T$ with $\epsilon = 10$ and $V_{\text{G}} = 200$. The simulations were run for $2 \times 10^4 \tau$ and the data used in the calculations was taken in the last $1.5 \times 10^3 \tau$, when the evolution was found to be in the stationary state in the centre of the box. For all data points, we used 100 samples to average the relevant quantities.

## PARTICLE DIFFUSION IN THE SPECKLE FIELD

We measured the particle's mean square displacement at late times in our simulations ($t > 1.5 \times 10^3 \tau$) and estimated the diffusion coefficient, $D$, from a linear fit of the time dependence of the mean square displacement. As can be seen in Fig. S2, the strong particles diffuse less than the weak ones, as they get trapped in the local minima of the random potential. Comparing these plots with Fig. 4, we find that higher diffusion coefficients correspond to lower $\langle \phi_6 \rangle$, when more defects are formed and the particles' packing is lower.

## EFFECTIVE SPECKLE PROPERTIES

We are interested in the limit where the dispersion in the speckle correlation function, $\sigma$, is of the same order as the particle size or smaller. Thus, to calculate the speckle-induced forces acting on a particle, we need to consider all intensities over the particle's cross-section. We can determine an effective speckle that, at each point, is the average intensity of the original speckle over a particle cross-section. This operation, smooths out the roughness of the intensity surface. This effect can be seen in Fig. S3, where it is clearly shown that the integration decreases the height of the intensity minima and increases the value of the lower intensity regions.

The statistical properties of the effective speckle are different from those of the original one. Figure S4 shows a comparison between the intensity distributions for dif-

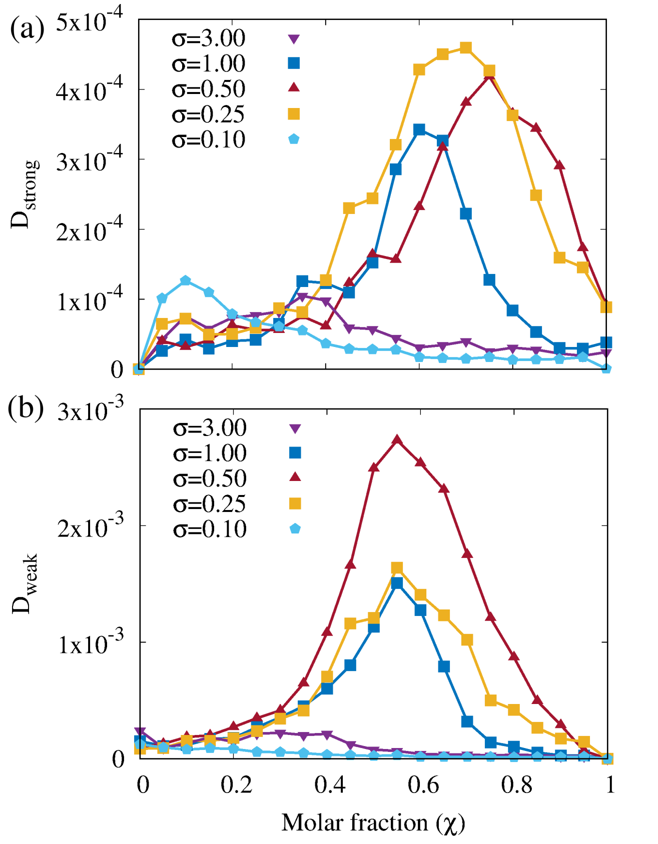


Supplementary Figure S2. (a) Strong and (b) weak particle diffusivity at late times in the same simulations as those shown in Fig. 4.

ferent $\sigma$ (histograms) and the original one (dashed line). For high $\sigma$, the averaging eliminates the highest intensities but hardly affects the distribution otherwise, as it remains approximately exponential. However, for lower $\sigma$, both high and low intensities are eliminated and the distribution is considerably affected. For the lowest $\sigma$, the intensities are narrowly distributed around a well-defined value.

The shape of the Gaussian intensity correlations also changes with the averaging. In particular, their dispersions increase. Figure S5 shows the dispersion of the correlations in the effective speckle, $\sigma_{\rm eff}$, as a function of the standard deviation of the original speckle, $\sigma$. The dashed line corresponds to $\sigma_{\rm eff} = \sigma$. For higher $\sigma$, the averaging does not change the dispersion significantly, because in this limit the features of the surface are, on average, larger than the particle size. For decreasing $\sigma$, $\sigma_{\rm eff}$ increases with respect to the original value, the speckle minima become wider and shallower, which leads to a lower effective force induced by the speckle on the particles.

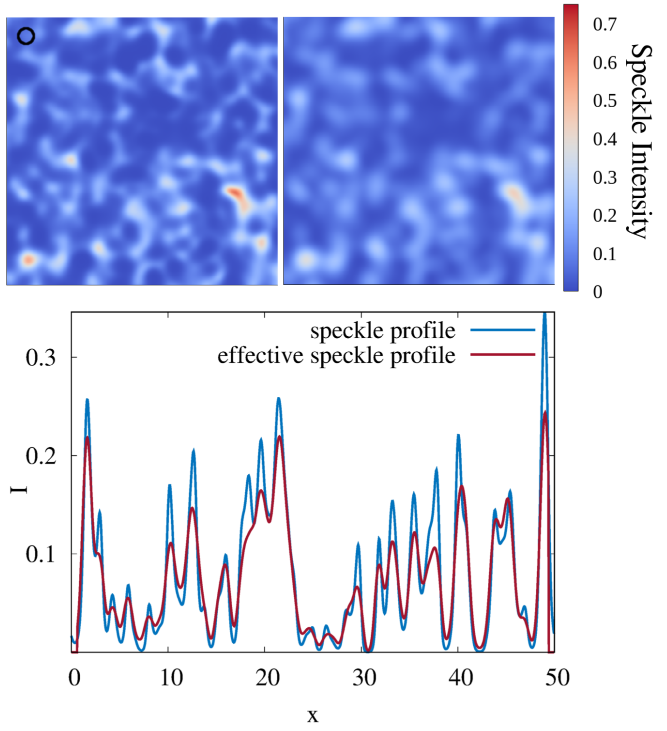


Supplementary Figure S3. Top left, the original speckle intensity surface; the black circle indicates the particle size. Top right, the effective speckle where each intensity point is an average of the intensities of the original one. Bottom, profile of the intensity surface of the original (blue) and the effective speckle (red) for $\sigma = 1$. The maximum speckle intensity is defined as the unit of intensity.

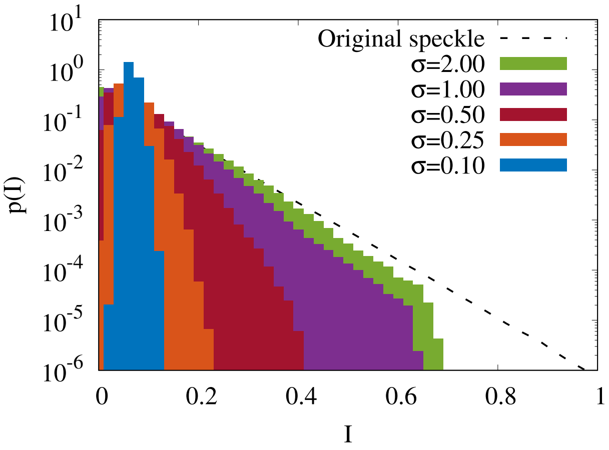


Supplementary Figure S4. Distribution of the speckle intensities of the effective speckles. 100 samples were used for each distribution. The dashed line corresponds to the original intensity distribution, for reference. The maximum speckle intensity is defined as the unit of intensity.

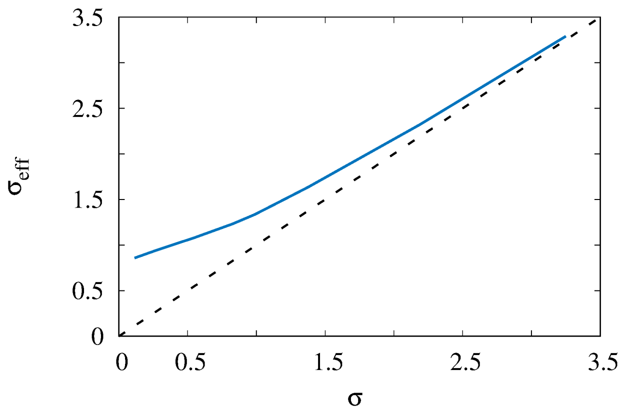


Supplementary Figure S5. Relation between the dispersion of the speckle correlation function in the original speckle and the corresponding dispersion measured in the effective speckle.

---

* contributed equally.
† nmaraujo@fc.ul.pt

[1] E. Pinçe, S. K. Velu, A. Callegari, P. Elahi, S. Gigan, G. Volpe, and G. Volpe, "Disorder-mediated crowd control in an active matter system," Nat. Commun. **7**, 10907 (2016).

[2] J. C. Crocker and D. G. Grier, "Methods of digital video microscopy for colloidal studies," J. Colloid Interfac. Sci. **179**, 298 (1996).

[3] A. P. Mosk, A. Lagendijk, G. Lerosey, and M. Fink, "Controlling waves in space and time for imaging and focusing in complex media," Nat. Photon. **6**, 283 (2012).

[4] G. Volpe, L. Kurz, A. Callegari, G. Volpe, and S. Gigan, "Speckle optical tweezers: Micromanipulation with random light fields," Opt. Express **22**, 18159 (2014).

[5] G. Volpe, G. Volpe, and S. Gigan, "Brownian motion in a speckle light field: tunable anomalous diffusion and selective optical manipulation," Sci. Rep. **4**, 3936 (2014).

[6] H. A. Makse, S. Havlin, M. Schwartz, and H. E. Stanley, "Method for generating long-range correlations for large systems," Phys. Rev. E **53**, 5445 (1996).

[7] E. A. Oliveira, K. J. Schrenk, N. A. M. Araújo, H. J. Herrmann, and J. S. Andrade, "Optimal-path cracks in correlated and uncorrelated lattices," Phys. Rev. E **83**, 046113 (2011).

[8] H.-O. Peitgen and D. Saupe, eds., *The Science of Fractal Images* (Springer-Verlag New York, Inc., New York, NY, USA, 1988).

[9] A. C. Brańka and D. M. Heyes, "Algorithms for brownian dynamics computer simulations: Multivariable case," Phys. Rev. E **60**, 2381 (1999).
